# Supplementary material for: Printable Nanocomposites with Superparamagnetic Maghemite ($\gamma$-Fe$_2$O$_3$) Particles for Microinductor-core Applications
Source: arXiv:2507.23522 source file (2025-07-31)
Supplement: Supplementary file 1 [file Article_2___Material_Paper__Supplementary___CleanVersion_.pdf]

# Supplementary information

## Printable Nanocomposites with Superparamagnetic Maghemite ($\gamma$-$Fe_2O_3$) Particles for Microinductor-core Applications


M. Zambach,[1] M. Varón,[1] T. Veile,[1] B. N. Sanusi,[2] M. Knaapila,[1,3] A. M. Jørgensen,[4] L. Almásy,[5] C. Johansson,[6] Z. Ouyang,[2] M. Beleggia,[4,7] and C. Frandsen[1,*]

[1]*DTU Physics, Technical University of Denmark, 2800 Kgs. Lyngby, Denmark*
[2]*DTU Electro, Technical University of Denmark, 2800 Kgs. Lyngby, Denmark*
[3]*Department of Physics, Norwegian University of Science and Technology, 7034 Trondheim, Norway*
[4]*DTU Nanolab, Technical University of Denmark, 2800 Kgs. Lyngby, Denmark*
[5]*Institute for Energy Security and Environmental Safety, HUN-REN Centre for Energy Research, 1121 Budapest, Hungary*
[6]*RISE Research Institute of Sweden, Sensor Systems, 417 55 Göteborg, Sweden*
[7]*Department of Physics, University of Modena and Reggio Emilia, 41125 Modena, Italy*



(Dated: July 24, 2025)


### FITTING PARAMETERS AND MODEL DESCRIPTION - SMALL ANGLE SCATTERING

To estimate the overall fraction of particles in the non-aggregated phase we fitted the scattering intensity profiles with a sum of two models. The first model handling the scattering from individual, non-aggregated particles and the second modelling the scattering from aggregated particles. The scattering intensity $I(Q)$ as function of scattering vector $Q$ is thus

$$I(Q) = \text{scale}_i\, \varphi_i\, P_i(Q)\, S_i(Q) + \text{scale}_a\, \varphi_a\, P_a(Q)\, S_a(Q) + \text{Background} \tag{1}$$

Here subscript $i$ and $a$ denote the models for the individual and aggregated models, 'scale' is the model weighting factor, $\varphi$ is the volume fraction of particles in the sample, $P(Q)$ is the model form factor, and $S(Q)$ is the model structure factor.

For the non-aggregated phase a spherical form-factor [1] with interaction from a hard-sphere structure factor was used [2**?** ]. The spherical form factor reads

$$P(Q) = (\Delta\rho)^2\; V_p\, \left[3\frac{\sin(QR_p) - QR_p\cos(QR_p)}{(QR_p)^3}\right]^2, \tag{2}$$

with $\Delta\rho$ being the difference in scattering length density and $V_p = \frac{4}{3}\pi R_p^3$ being the particle volume of a particle with radius $R_p$,

The hard-sphere structure factor factor for the non-aggregated particles is given [2**?** ]

$$S_i(Q) = 1 + \frac{\varphi}{V_p}\int_0^\infty \left[g(r,\varphi,R_{eff}) - 1\right]\frac{\sin(Qr)}{Qr}4\pi r^2 dr, \tag{3}$$

where a Percus-Yevick hard-sphere correlation function $g(r,\varphi,R_{eff})$ used with particle center distance $r$, effective particle radius $R_{eff}$ [2**?** ].

For the aggregated particles scattering was modelled by a fractal model using spherical particle form factor as in (2) and a fractal structure factor [3]. The fractal structure factor reads

$$S_a(Q) = 1 + \frac{D_f\Gamma(D_f - 1)}{\left[1 + \left(\frac{1}{Q\xi}\right)^2\right]^{\frac{D_f-1}{2}}}\frac{\sin\left[(D_f - 1)\tan^{-1}(Q\xi)\right]}{(QR_p)^{D_f}}, \tag{4}$$


* Contact author: fraca@fysik.dtu.dk

with $D_f$ being the fractal dimension, $\Gamma(x)$ being the Gamma function of $x$, and $\xi$ being the fractal correlation length [3].

For all models a pin-hole smearing of 0.18-0.2 was used together with a particle polydispersity of 0.15. The scattering length density for maghemite in Polyvinyl alcohol at the used neutron wavelengths is $\Delta\rho_a = \Delta\rho_i = (6.68 \times 10^{-6}$ Å$^{-2}$ - $0.566 \times 10^{-6}$ Å$^{-2}) = 6.114 \times 10^{-6}$ Å$^{-2}$. Model fit values can be seen in table I below. Weight of the two models is extracted as the product of scale times the volume fraction of one model divided by the sum of the product of the scale and volume fractions of both models. For all measurements the absolute scale was calibrated by the incoherent scattering of water, intensity was normalised to sample thickness and background was corrected by subtraction of blank polymer measurement. The three different $Q$-ranges (from varying detector distance and wavelength) were radially integrated and then merged [4].

TABLE I: Fitting parameters used for small angle scattering fitting of the 6 different samples. Polydispersity was fixed to 0.15 of radius. Radii based on volume weighted lognormal distribution with distribution width noted after the ± symbol.

| **Sample Particle Content** | **Fractal Model** | | | | | **Hardsphere Model** | | | |
|---|---|---|---|---|---|---|---|---|---|
| | scale$_a$ | Vol. frac. $\varphi_a$ | Radius $R_{p,a}$ [nm] | Fract. Dim. $D_f$ | Fract. corr. Length $\xi$ [nm] | scale$_i$ | Vol. frac. $\varphi_i$ | Radius [nm] $R_{p,i}$ [nm] | Eff. Radius $R_{eff}$ [nm] |
| 1 Vol% | 0.125 | 0.01 | 8.0±1.2 | 3 | 15 | 0.02 | 0.01 | 7.6±1.1 | 7.6±1.1 |
| 4.5 Vol% | 0.0175 | 0.05 | 6.9±1.0 | 3 | 10 | 0.11 | 0.07 | 7.3±1.1 | 9.5±1.4 |
| 10.1 Vol% | 0.2 | 0.1 | 6.9±1.0 | 3 | 8 | 0.2 | 0.15 | 6.9±1.0 | 7.8±1.2 |
| 17.7 Vol% | 0.08 | 0.20 | 7.1±1.1 | 3 | 13.5 | 0.38 | 0.28 | 7.1±1.1 | 7.6±1.1 |
| 35.3 Vol% | 0.03 | 0.36 | 6.9±1.0 | 3 | 14.5 | 0.56 | 0.36 | 7.0±1.1 | 7.2±1.1 |
| 44.7 Vol% | 0.043 | 0.445 | 7.0±1.1 | 1.8 | 50 | 1.00 | 0.445 | 7.2±1.1 | 7.2±1.1 |

## AC-SUSCEPTIBILITY FITTING MODEL

Particle susceptibility is calculated by a combination of the Debye-model including separate relaxation times for the parallel and perpendicular directions [5, 6]. Parallel and perpendicular particle susceptibility are

Parallel:
$$\chi_{\mathrm{p},||} = \epsilon_{\mathrm{M}} \frac{R'}{R} \frac{1}{1 + i\omega\tau_{||}} \tag{5a}$$

with
$$\tau_{||} = \begin{cases} \tau_0\, 2R'/(R - R') & \text{for } \epsilon_{\mathrm{k}} \leq 2, \\ \tau_0 \sqrt{\pi}\, \exp(\epsilon_{\mathrm{k}})/(2\epsilon_{\mathrm{k}}^{3/2}) & \text{for } \epsilon_{\mathrm{k}} > 2, \end{cases} \tag{5b}$$

Perpendicular:
$$\chi_{\mathrm{p},\perp} = \frac{\epsilon_{\mathrm{M}}}{2} \left[1 - R'/R\right] \frac{1}{1 + i\omega\tau_{\perp}} \tag{6a}$$

with
$$\tau_{\perp} = \tau_0\, 2\,(R - R')\,/\,(R + R') \quad \text{for all } \epsilon_{\mathrm{k}}, \tag{6b}$$

with $\tau_0$ being the attempt time, $\epsilon_{\mathrm{k}} = \frac{K_{\mathrm{u}} V}{k_B T}$, $K_{\mathrm{u}}$ the effective uniaxial particle anisotropy, $\epsilon_{\mathrm{M}} = \frac{\mu_0 V M_{\mathrm{s}}^2}{k_B T}$, where $V$ is the particle volume, $M_{\mathrm{s}}$ is the saturation magnetisation of the particle, $T$ is the temperature. The anisotropy weighting factors $R$ and $R'$ are

$$R = \int_0^1 \exp\left(\epsilon_{\mathrm{k}} x^2\right) \mathrm{d}x, \tag{7a}$$

$$R' = \int_0^1 x^2 \exp\left(\epsilon_{\mathrm{k}} x^2\right) \mathrm{d}x. \tag{7b}$$

The random orientation susceptibility is then

Random:
$$\chi_{\mathrm{p,R}} = \frac{1}{3}\chi_{\mathrm{p},||} + \frac{2}{3}\chi_{\mathrm{p},\perp}. \tag{8}$$

## HYSTERESIS LOOPS FOR POWER LOSS CALCULATIONS

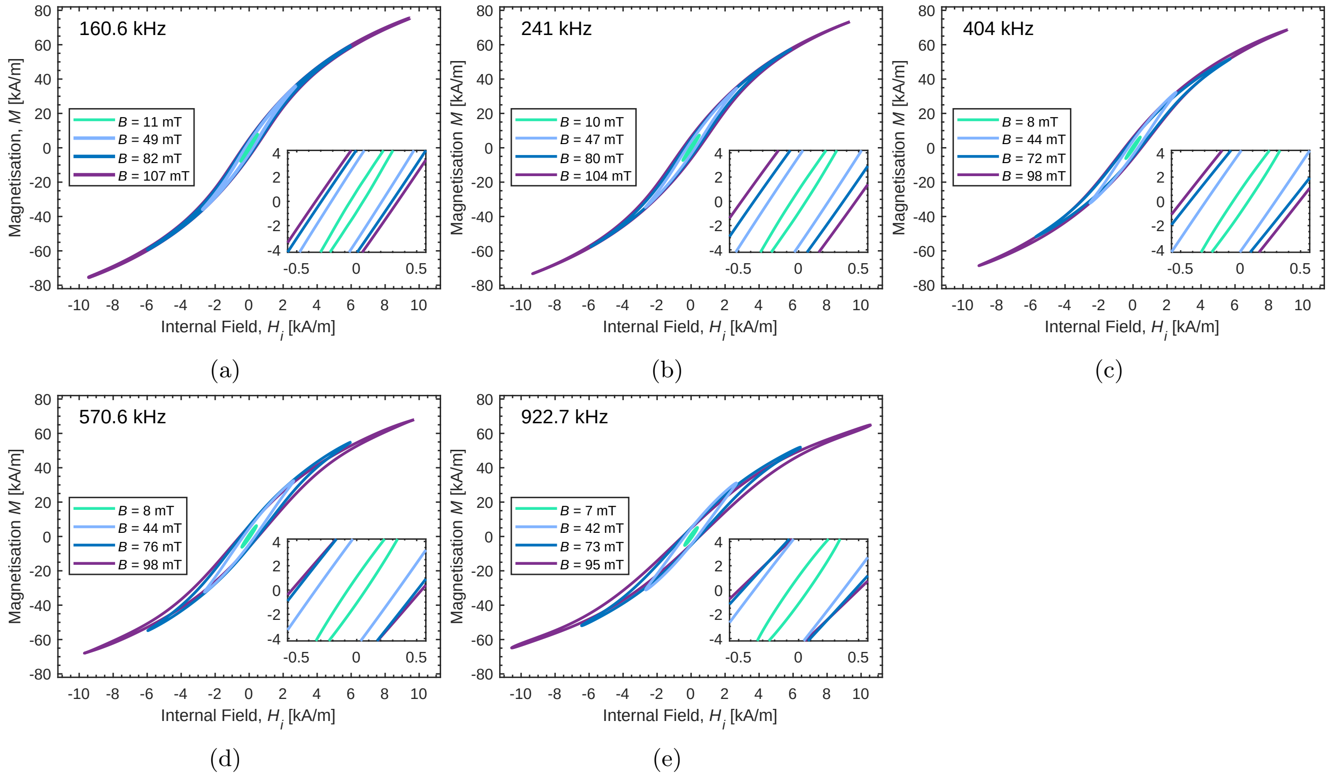


FIG. 1: Demagnetisation corrected high-frequency hysteresis curves for 44.7 vol% sample obtained at 160.6 kHz (a), 241 kHz (b), 404 kHz (c), 570.6 kHz (d) and 922.7 kHz (e) for applied fields of 0.8, 4, 8, and 12 kA/m.


[1] G. Fournet and A. Guinier, Theory of scattering of x-rays at small angles, Journal De Physique Et Le Radium **11**, 516 (1950).

[2] M. Kotlarchyk and S. Chen, Analysis of Small-Angle Neutron-Scattering Spectra from Polydisperse Interacting Colloids, Journal of Chemical Physics **79**, 2461 (1983).

[3] J. Teixeira, Small-Angle Scattering by Fractal Systems, Journal of Applied Crystallography **21**, 781 (1988).

[4] L. Almásy, New Measurement Control Software on the Yellow Submarine SANS Instrument at the Budapest Neutron Centre, Journal of Surface Investigation **15**, 527 (2021).

[5] M. Zambach, Z. Ouyang, M. Knaapila, M. Beleggia, and C. Frandsen, Design of superparamagnetic nanoparticle-materials for high-frequency inductor cores (2024), arXiv:2308.13407 [cond-mat.mes-hall].

[6] P. Svedlindh, T. Jonsson, and J. L. García-Palacios, Intra-potential-well contribution to the AC susceptibility of a noninteracting nano-sized magnetic particle system, Journal of Magnetism and Magnetic Materials **169**, 323 (1997).
